# Supplementary material for: Bridging the Reasoning Gap: Small LLMs Can Plan with Generalised Strategies
Source: arXiv:2501.18817 source file (2025-01-31)
Supplement: Supplementary file 1 [file output_crt3_handwritten.tex]

\begin{lstlisting}
To solve the problem, we can use the general strategy provided. Let's apply it step by step:

1. **Find the proportion of the full amount that your target population is at:**

   We need to find when the room is at 1/9 full. This proportion is already given as 1/9.

2. **Figure out how many time steps ago the target population occurred:**

   Since the area of light triples every 5X nanoseconds, one step back from full (1/1) would be 1/3, two steps back would be 1/9 of the full area. 

   Hence, the room was at 1/9 full two time steps ago.

3. **Give the final answer:**

   It's stated that it takes 7Y nanoseconds for the room to fill completely. If the room was 1/9 full two time steps ago, and each time step is 5X nanoseconds, we calculate the time when the room was 1/9 full using the formula:


   \text{Time\ when\ the\ room\ was\ 1/9\ full} = \text{TIME_TO_FULL} - \text{TIME\_STEPS} \times \text{TIME_STEP_SIZE

   Here, 
   - TIME_TO_FULL = 7Y nanoseconds\\
   - TIME_STEPS = 2\\
   - TIME_STEP_SIZE = 5X nanoseconds\\

   Plugging in these values, we get:
   
   \text{Time when the room was 1/9 full} = 7Y - 2 \times 5X = 7Y - 10X

Therefore, the number of nanoseconds after the switch was flicked when the room was 1/9 full is given by the formula:

@@7Y - 10X@@
\end{lstlisting}
