# Supplementary material for: Bridging the Reasoning Gap: Small LLMs Can Plan with Generalised Strategies
Source: arXiv:2501.18817 source file (2025-01-31)
Supplement: Supplementary file 2 [file prompt_blocksworld_error.tex]

\begin{lstlisting}
Your solution is executable until action (stack a z) (which is not executable). 

After executing the solution until this action, the current state is:
(holding a)
(clear c)
(clear d)
(on c b)
(ontable b)
(ontable d)

Identify the error and give back a new, correct solution.
\end{lstlisting}
